# Supplementary material for: Distributional Model Equivalence for Risk-Sensitive Reinforcement Learning
Source: arXiv:2307.01708 source file (2023-12-03)
Supplement: Supplementary file 1 [file planning-algorithms-used.tex]

\section{Planning algorithms used}\label{sec:PlanningAlgoUsed}

\begin{algorithm}
   \caption{Mean-variance value iteration}
\begin{algorithmic}
   \STATE {\bfseries Input:} Variance weight $\lambda$, error threshold $\theta$, MDP $(\stateSpace,\actionSpace,\transitionFn,\rewardFn,\gamma)$
   \STATE Initialize $V(x) = 0$ for all $x\in\stateSpace$.
   \STATE Initialize ${Var}(x) = 0$ for all $x\in\stateSpace$.
   \REPEAT
   \FOR{each $x\in \stateSpace$}
   \STATE $V_{tmp}(x,a) = \E_{R\sim \rewardFn(x,a)}\left[R\right]+\gamma \sum_{x'\in\stateSpace}\transitionFn(x'|x,a)\,V(x')$\vspace{3pt}
   \STATE $Var_{tmp}(x,a) = \E_{R\sim \rewardFn(x,a)}\left[R^2\right]+2\gamma \sum_{x'\in\stateSpace}\transitionFn(x'|x,a)\,V(x')+\gamma^2\sum_{x'\in\stateSpace}\transitionFn(x'|x,a)\,Var(x')$\vspace{3pt}
    \STATE $meanVar(x,a) = V_{tmp}(x,a)-\lambda Var_{tmp}(x,a)$\vspace{3pt}
    \STATE $\pi(x) = \arg\max_{a\in \actionSpace}meanVar(x,a)$\vspace{3pt}
    \STATE $V_{old}(s) = V(s)$\vspace{3pt}
    \STATE $Var_{old}(s) = Var(s)$\vspace{3pt}
    \STATE $V(s)=V_{tmp}(\pi(s))$\vspace{3pt}
    \STATE $Var(s)=Var_{tmp}(\pi(s))$\vspace{3pt}
    \STATE $\Delta =\max(\Delta, |Var(s)-Var_{old}(s)|, |V(s)-V_{old}(s)|)$
   \ENDFOR
   \UNTIL{$\Delta < \theta$}
   \STATE {\bf return} $\pi$
\end{algorithmic}
\end{algorithm}

\begin{algorithm}
   \caption{CVaR value iteration}
\begin{algorithmic}
   \STATE {\bfseries Input:} Level $\tau$, number of iterations $num_iters$, probability distribution representation $\F$, projection $\Pi_\F$, discretization width $\varepsilon$, MDP $(\stateSpace,\actionSpace,\transitionFn,\rewardFn,\gamma)$ with reward bound $R_{\text{max}}$, starting state $x_0$\vspace{4pt}
   \STATE Let $\B_\varepsilon$ be a discretization of $[-R_{\text{max}}/(1-\gamma),R_{\text{max}}/(1-\gamma)]$ into intervals of length $\varepsilon$
   \STATE Initialize $\eta(x,a,b) = \Pi_\F\delta_0$ for all $x\in\stateSpace$, $a\in\actionSpace$, $b\in \B_\varepsilon$
   \STATE $b=0$
   \STATE $k=0$
   \REPEAT
   \FOR{each $x\in \stateSpace$}
   % \STATE $G(x,a)=\E[\eta(x,a,b)]$
   \STATE $a'=\arg\min_{a\in\actionSpace}\left[\max(b-\frac1\tau \E_{Z\sim \eta(x,a,b)}[Z],0)\right]$
   \FOR{each $a\in \actionSpace$}
   \STATE $\eta(x,a,b)=\Pi_\F\left(\sum_{x'\in\stateSpace}\transitionFn(x'|x,a)\,\E_{R\sim \rewardFn(x,A)}\left[(b_{,\gamma})_{\#}\eta(x', a', b)\right]\right)$
   \vspace{3pt}
    \ENDFOR
    \STATE $V_{old}(s) = V(s)$\vspace{3pt}
    \STATE $Var_{old}(s) = Var(s)$\vspace{3pt}
    \STATE $V(s)=V_{tmp}(\pi(s))$\vspace{3pt}
    \STATE $Var(s)=Var_{tmp}(\pi(s))$\vspace{3pt}
    \STATE $\Delta =\max(\Delta, |Var(s)-Var_{old}(s)|, |V(s)-V_{old}(s)|)$
   \ENDFOR
   \UNTIL{$k = num_iters$}
   \STATE {\bf return} $\pi$
\end{algorithmic}
\end{algorithm}
